# Supplementary material for: UniVS: Unified and Universal Video Segmentation with Prompts as Queries
Source: arXiv:2402.18115 source file (2024-06-10)
Supplement: Supplementary file 1 [file sepsa_training.tex]

\begin{table}[!t]
\centering
\begin{subtable}{0.45\textwidth}
\centering
\small
\setlength{\tabcolsep}{0.5mm}{
    \linespread{2}
    \begin{tabular}{p{0.18\textwidth}<{\centering}p{0.13\textwidth}<{\centering}p{0.13\textwidth}<{\centering}p{0.15\textwidth}<{\centering}p{0.13\textwidth}<{\centering}p{0.15\textwidth}<{\centering}}
    \Xhline{0.8pt}
    Self-Attn & \multicolumn{5}{c}{PVOS}  \\ 
    \cline{2-6}
    Type & G$^{th \& sf}$ & G$^{th}_{seen}$  & G$^{th}_{unseen}$  & G$^{sf}_{seen}$ & G$^{sf}_{unseen}$ \\
    \Xhline{0.8pt}
    SepSA   & 57.9 & 58.4 & 55.0 & 63.5 & 54.5 \\
    SepSA-e & 61.8 & 59.7 & 57.1 & 68.2 & 62.1 \\
    SepSA-l & 48.5 & 41.0 & 46.5 & 51.0 & 55.5 \\
    \Xhline{0.8pt}
    \end{tabular}
    }
    \caption{\small Quantitative performance comparison}
    \vspace{+2mm}
\end{subtable}
\begin{subfigure}{0.48\textwidth}
    \centering
    \includegraphics[width=0.95\textwidth]{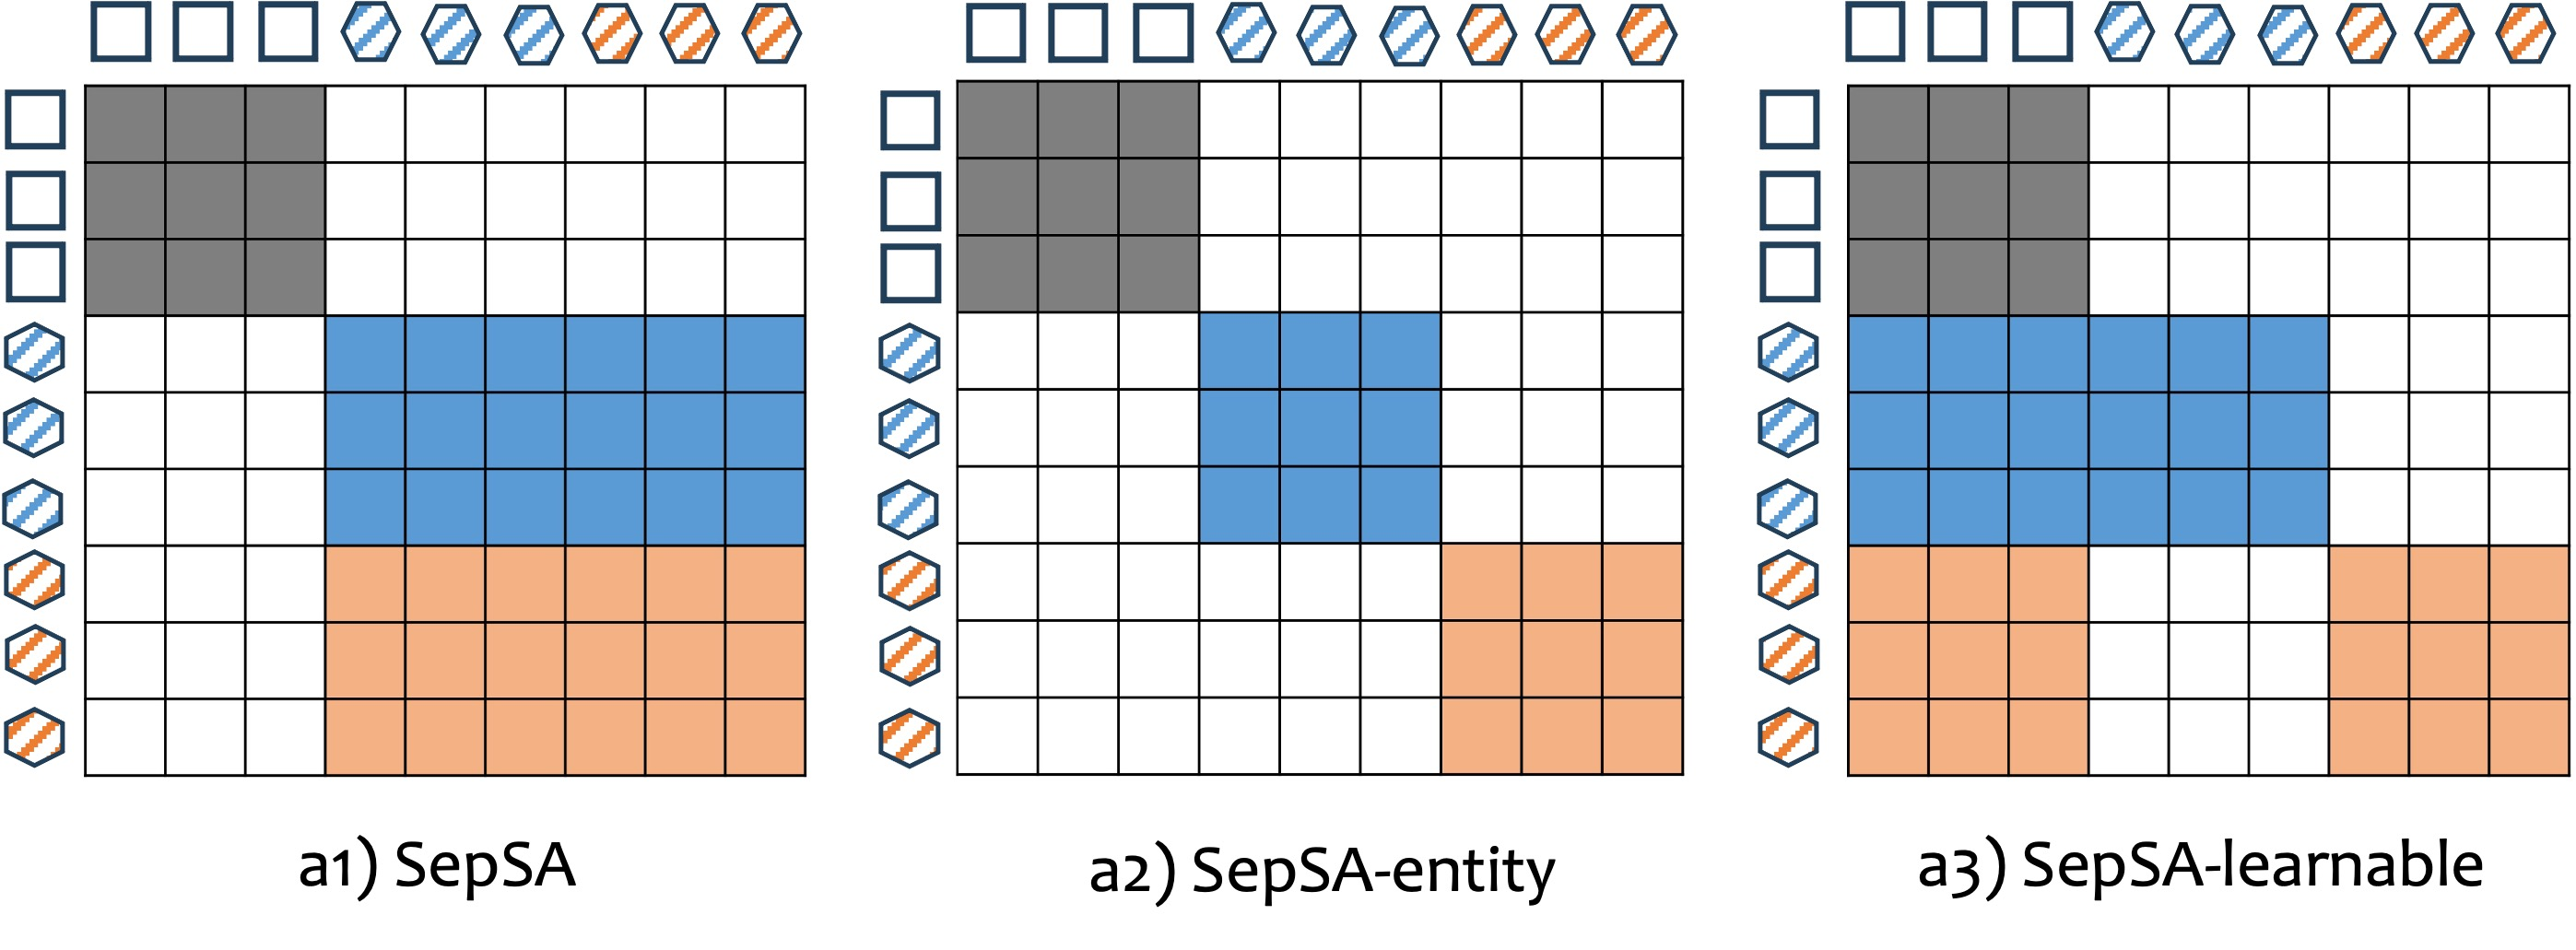}
    \vspace{-2mm}
\end{subfigure}
\caption{\small Ablation study on PVOS tasks. 
} \label{tab:sepsa_refer}
\vspace{-1mm}
\end{table}
