# Supplementary material for: UniVS: Unified and Universal Video Segmentation with Prompts as Queries
Source: arXiv:2402.18115 source file (2024-06-10)
Supplement: Supplementary file 2 [file sota_open_voc.tex]

\begin{table}[!b]
\begin{subtable}{0.495\textwidth}
\small
\setlength{\tabcolsep}{1.45mm} 
    \begin{tabular}{cc|ccc}
    \Xhline{0.8pt}
     \!\!Model & Backbone & HOTA$_{482}$ & HOTA$_{78}$  & \!HOTA$_{404}$ \\
    \hline
    \!\!MinVIS  & R50    & 1.35 & 5.50 & 0.49  \\
    \!\!MinVIS  & SwinL  & *    & *    & 14.6  \\
    \!\!OpenVIS & R50    & 3.48 & 5.81 & 3.0   \\
    \!\!OpenVIS & SwinL  & *    & *    & 23.4  \\
    \!\!UniVS   & R50    &      \\
    \!\!UniVS   & SwinL  &      \\
    \Xhline{0.8pt}
\end{tabular}
\caption{\small Open-vocabulary VIS benchmarks}
\end{subtable}
\begin{subtable}{0.495\textwidth}
\small
\setlength{\tabcolsep}{1.45mm} 
    \begin{tabular}{cc|ccc}
    \Xhline{0.8pt}
      \!\!Model & Backbone & OWTA$_{482}$ & OWTA$_{78}$  & \!OWTA$_{404}$ \\
    \hline
    \!\!OWTB      &        & 55.8 & 59.8 & 38.8 \\
    \!\!DEVA+M2F  & R50    &  \\
    \!\!DEVA+M2F  & SwinL  &  \\
    \!\!UniVS     & R50    &      \\
    \!\!UniVS     & SwinL  &      \\
    \Xhline{0.8pt}
\end{tabular}
\caption{\small Open-vocabulary VOS benchmarks}
\end{subtable}
\vspace{-5mm}
\caption{\small Performance comparison on open-vocabulary VS benchmarks, BURST and UVO datasets. `com' refers to the 78 common categories that overlap with COCO dataset, while `unc' indicates the 404 uncommon categories.
} \label{tab:open_voc}
\vspace{-2mm}
\end{table}
