# Supplementary material for: UniVS: Unified and Universal Video Segmentation with Prompts as Queries
Source: arXiv:2402.18115 source file (2024-06-10)
Supplement: Supplementary file 3 [file vs_datasets.tex]

\begin{table*}[h]
\begin{subtable}{0.95\textwidth}
\centering
\small
\setlength{\tabcolsep}{2.0mm}
    \begin{tabular}{c|ccc|c|c|c}
    \Xhline{0.8pt}
    % \rowcolor{isabelline}
     Tasks & \multicolumn{3}{c|}{VIS} & VSS & VPS & PVOS \\
     % \cline{2-6}
     Datsets & \cellcolor{LightYellow} \!\!YTVIS19 & \cellcolor{LightYellow}\!\!YTVIS21 & \cellcolor{lightmauve} OVIS & \cellcolor{LightCyan} VSPW & \cellcolor{LightCyan} VIPSeg  & \cellcolor{LightCyan} \!\!VIPOSeg \\
    \hline
    Videos   & 2238/302/343 & 2985/421/453  & 670/140/154 & 2806/343/387 & 2806/343/387 & 2806/343/387 \\ % 4x
    Images   & 97k  & 92k  & 51k  & 252k & 85k  & 85k  \\  
    Masks    & 131k & 232k & 296k &  -   & 926k & 926k  \\
    Classes  &  40 &  40 & 25 & 124      & 124  & 124   \\ % 3x
    Thing    & $\checkmark$ & $\checkmark$ & $\checkmark$ & $\checkmark$ & $\checkmark$ & $\checkmark$  \\
    Stuff    & \crossmark   & \crossmark   & \crossmark   & $\checkmark$ & $\checkmark$ & $\checkmark$  \\
    Exhaustive & \crossmark & \crossmark   & \crossmark   & $\checkmark$ & $\checkmark$ & $\checkmark$  \\
    \Xhline{0.8pt}
    \end{tabular}
    \caption{\small VIS/VSS/VPS and PVOS datasets
    }\label{tab:vs_data1}
\end{subtable}
\begin{subtable}{0.95\textwidth}
\centering
\small
\setlength{\tabcolsep}{1.8mm} 
    \begin{tabular}{c|cccccc|cc}
    \Xhline{0.8pt}
    % \rowcolor{isabelline}
     Tasks & \multicolumn{6}{c|}{VOS} & \multicolumn{2}{c}{RefVOS}\\
     % \cline{2-8}
     Datasets & \cellcolor{cottoncandy}\!DAVIS & \cellcolor{LightYellow} \!YTVOS & \cellcolor{lightmauve} \!\!MOSE & \!\!BURST & \!UVO$_D$ & \!UVO$_S$ & \cellcolor{cottoncandy}\!RefDAVIS & \cellcolor{LightYellow} RefYTVOS \\
    \hline
    Videos   & 60/30/-  & 3471/474/508  & 1507/311/331 & 500/993/1421 & 1024 & 10k & 60/30/- & \!3471/202/305 \\ % 4x
    Images   &  6k       & 97k           & 96k   & 196k & 93k  & 31k  & 6k   & 97k  \\
    Masks    &  13k      & 197k          & 431k  & 600k & -    & -    & 13k  & 197k  \\
    Classes  & -         & 94            & 36    & 482  & open & open & -    & - \\ % 3x
    Expression & - & - & - & - & - & - & 1.5k & 28k \\
    Thing    & $\checkmark$  & $\checkmark$  & $\checkmark$ & $\checkmark$ & $\checkmark$ & $\checkmark$ & $\checkmark$ & $\checkmark$ \\
    Stuff    & \crossmark    & \crossmark    & \crossmark   & \crossmark   & \crossmark   & \crossmark   & \crossmark & \crossmark \\
    Exhaustive & \crossmark    & \crossmark    & \crossmark   & \crossmark   & ($\checkmark$) & ($\checkmark$)   & \crossmark & \crossmark \\ % 1x
    \Xhline{0.8pt}
    \end{tabular}
    \caption{\small VOS and RefVOS datasets
    }\label{tab:vs_data2}
\end{subtable}
\vspace{-2mm}
\caption{ Statistics for video segmentation datasets, including VIS, VSS, VPS, PVOS, VOS, and RefVOS tasks. `($\checkmark$)' indicates that this dataset provides exhaustive annotations only for thing classes. These datasets covered by the same color share the source video data but have different annotation formats, such as VSPW, VIPSeg and VIPOSeg.
} \label{tab:training_details}
\end{table*}
